# Supplementary material for: Improving Calibration in Deep Metric Learning With Cross-Example Softmax
Source: arXiv:2011.08824 source file (2020-11-17)
Supplement: Supplementary file 1 [file appendix.tex]

\section{Experimental setup}
\label{sec:appx_setup}

\section{Proofs}
\label{sec:appx_proofs}
\begin{proof}[Proof of Lemma~\ref{lem:churn-err}]
Recall from Definition~\ref{def:churn-two-models} that 
\begin{align}
\churn{w_1, w_2} &= \mathbb{P}_{\X}\big[\hat{\Y}_{\X, w_1} \neq \hat{\Y}_{\X, w_2}\big] = \mathbb{P}_{\X, \Y}\big[\hat{\Y}_{\X, w_1} \neq \hat{\Y}_{\X, w_2}\big] \nonumber \\
&\overset{}{=}\mathbb{P}_{\X, \Y}\big[\{\hat{\Y}_{\X, w_1} = \Y, \hat{\Y}_{\X, w_2} \neq \Y\} \cup \{\hat{\Y}_{\X, w_1} \neq \Y, \hat{\Y}_{\X, w_1} \neq \hat{\Y}_{\X, w_2} \}\big] \nonumber \\
&\overset{(i)}{\leq}\mathbb{P}_{\X, \Y}\big[\hat{\Y}_{\X, w_1} = \Y, \hat{\Y}_{\X, w_2} \neq \Y \big]  + \mathbb{P}\big[\hat{\Y}_{\X, w_1} \neq Y, \hat{\Y}_{\X, w_1} \neq \hat{\Y}_{\X, w_2}\big] \nonumber \\
&\overset{(ii)}{\leq} \mathbb{P}\big[\hat{\Y}_{\X, w_2} \neq \Y\big] + \mathbb{P}\big[\hat{\Y}_{\X, w_1} \neq \Y\big] \nonumber \\
& = \perr{w_2} + \perr{w_1},
\end{align}
where $(i)$ and $(ii)$ follow from the union bound and the fact that $\mathbb{P}[A] \leq \mathbb{P}[B]$ whenever $A \subseteq B$, respectively.
\end{proof}

\begin{proof}[Proof of Lemma~\ref{lem:churnR-kl}]
It is clear from \eqref{eq:churn-random-collision} that $\churnR{w_1, w_2}$ is a monotonic function of $$\mathbb{E}_{\X}\big[- \log \sum_{j \in \mathscr{Y}} f(\X; w_1)_j f(\X; w_2)_j\big].$$
Now, using Jensen's inequality, we get that 
\begin{align}
\label{eq:collision-proxy-1-1}
\mathbb{E}_{\X}\big[- \log \sum_{j \in \mathscr{Y}} f(\X; w_1)_j f(\X; w_2)_j\big] &\leq \mathbb{E}_{\X}\big[- \sum_{j \in \mathscr{Y}}f(\X; w_1)_j\log f(\X; w_2)_j\big] \nonumber \\
& = \mathbb{E}_{\X}\big[H\big(f(X; w_1), f(X;w_2)\big)\big],
\end{align}
where, for two distributions $p$ and $q$, $H(p, q)$ denotes the cross entropy between $p$ and $q$. Using similar argument, we get that
\begin{align}
\label{eq:collision-proxy-1-2}
\mathbb{E}_{\X}\big[- \log \sum_{j \in \mathscr{Y}} f(\X; w_1) f(\X; w_2)\big] &\leq \mathbb{E}_{\X}\big[H\big(f(\X; w_2), f(\X;w_1)\big)\big],
\end{align}
It follows from \eqref{eq:collision-proxy-1} and \eqref{eq:collision-proxy-1-2} that \eqref{eq:collision-proxy-1} serves as a proxy for $\churnR{w_1, w_2}$. Note that \eqref{eq:collision-proxy-1} is equivalent to \eqref{eq:collision-proxy-2}, as we have
$$
\KL(p, q) = H(p, q) - H(p).
$$
\end{proof}

\begin{proof}[Proof of Lemma~\ref{lemm:churn-margin}]
Note that, for any $j \neq \hat{y}_{x, w_1}$,
\begin{align}
\label{eq:tv-churn-confidence-1}
&f(x; w_2)_{\hat{y}_{x, w_1}} - f(x; w_2)_j \nonumber \\
&\qquad = f(x; w_2)_{\hat{y}_{x, w_1}} - f(x; w_1)_{\hat{y}_{x, w_1}} + \underbrace{f(x; w_1)_{\hat{y}_{x, w_1}} - f(x; w_1)_j}_{\geq \gamma_{x, w_1}} \; + f(x; w_1)_j - f(x; w_2)_j \nonumber \\
&\qquad \geq \gamma_{x, w_1} - \sum_{j \in \mathscr{Y}} |f(x;w_1)_j - f(x;w_2)_j| \nonumber \\
&\qquad = \gamma_{x, w_1} - \TV\big(f(x;w_1), f(x;w_2)\big).
\end{align}
Similarly, for any $j \neq \hat{y}_{x, w_2}$, we can establish that
\begin{align}
\label{eq:tv-churn-confidence-2}
f(x; w_1)_{\hat{y}_{x, w_2}} - f(x; w_1)_j \geq \gamma_{x, w_2} - \TV\big(f(x;w_1), f(x;w_2)\big).
\end{align}
Note that experience churn between the two models on $x$ is equivalent to 
\begin{align}
\label{eq:tv-churn-confidence-3}
&\{\hat{y}_{x, w_1} \neq \hat{y}_{x, w_2}\} \subseteq \nonumber \\
&\qquad \big\{\exists j \neq \hat{y}_{x, w_1} : f(x; w_2)_{\hat{y}_{x, w_1}} < f(x; w_2)_j\big\} \bigcup \big\{\exists j \neq \hat{y}_{x, w_2} : f(x; w_1)_{\hat{y}_{x, w_2}} < f(x; w_1)_j\big\} \nonumber \\
& \qquad \overset{(i)}{\subseteq}  \big\{ \TV\big(f(x; w_1), f(x; w_2)\big) > \gamma_{x, w_1}\big\} \bigcup \big\{ \TV\big(f(x; w_1), f(x; w_2)\big) > \gamma_{x, w_2}\big\},
\end{align}
where $(i)$ follows from \eqref{eq:tv-churn-confidence-1} and \eqref{eq:tv-churn-confidence-2}. Now, \eqref{eq:tv-churn-confidence-3} implies that
\begin{align}
\mathbb{P}_{\X}{\{\hat{\Y}_{\X, w_1} \neq \hat{\Y}_{\X, w_2}\}} \leq \mathbb{P}_{\X}\big[\TV(f(\X; w_1), f(\X; w_2)) > \min\{\gamma_{\X, w_1}, \gamma_{\X, w_2}\}\big].
\end{align}
\end{proof}

\begin{proof}[Proof of Theorem \ref{thm:entropy}]
Let the prediction for a given $x$ be $p = \modelB{x}$. W.L.O.G. let $p \geq 1-p$.  The prediction confidence is then $$\gamma_{x, w^*} = p - (1-p) = 2p-1.$$
Now we can write entropy in terms of the prediction confidence \begin{align*}
\entropy(\modelB{x}) &= -p \log(p) - (1-p)\log(1-p) \\
&= -\frac{(1+\gamma_{x, w^*})}{2} \times \log \left(\frac{1+\gamma_{x, w^*}}{2}\right) -\frac{(1-\gamma_{x, w^*})}{2} \times\log \left(\frac{1-\gamma_{x, w^*}}{2} \right) \\
& \triangleq g(\gamma_{x, w^*}).
\end{align*} 
Now the gradient of $g(.)$ is $\nabla g(\gamma_{x, w^*}) = \frac{1}{2}\log\left(\frac{1-\gamma_{x, w^*}}{1+\gamma_{x, w^*}} \right)$, which is less than $0$ for $\gamma_{x, w^*} \in [0, 1]$. Hencee, the function $g(\gamma_{x, w^*})$ is a decreasing function for inputs in range $[0, 1]$. Hence, if $g(\gamma_{x, \widetilde{w}}) \leq g(\gamma_{x, w^*})$ implies $\gamma_{x, \widetilde{w}} \geq \gamma_{x, w^*}$. 
\end{proof}

\begin{proof}[Proof of Lemma \ref{lem:entropy}]
Assume that \begin{equation*}
    \mathbb{E}_{\mathsf{X}}\left[ \entropy(\modelE{x}) \right] > \mathbb{E}_{\mathsf{X}}\left[  \entropy(\modelB{x}) \right].
\end{equation*} Since $\modelB{\cdot}$ is the minimizer of Loss \eqref{eq:population_risk}, \begin{equation*}
    L(\modelB{x}, y) < L(\modelE{x}, y).
\end{equation*} Combining these two gives us \begin{equation*}
    L_{entropy}\big(\mathbb{P}_{\mathsf{X}, \mathsf{Y}}; \modelB{x}\big) < L_{entropy}\big(\mathbb{P}_{\mathsf{X}, \mathsf{Y}}; \modelE{x}\big),
\end{equation*} which contradicts that $\modelE{\cdot}$ is a minimizer of the Loss \eqref{eq:entropy_loss}. Hence $\mathbb{E}_{\mathsf{X}}\left[\entropy(\modelE{x}) \right]  \leq \mathbb{E}_{\mathsf{X}}\left[ \entropy(\modelB{x}) \right] .$
\end{proof}

\begin{proof}[Proof of Lemma~\ref{lemm:churn-hellinger-tv}]
%\begin{remark}[Connecting $\churnR{w_1, w_2}$ to other distance measures]
Given two distributions $p, q \in \Delta^{K}$, the Hellinger distance between $p$ and $q$ is defined as follows. 
\begin{align}
\label{eq:hellinger}
\hellinger{p, q} = \frac{1}{\sqrt{2}}\sqrt{\sum_{j}(\sqrt{p_j} - \sqrt{q_j})^2}.
\end{align}
or 
\begin{align}
\label{eq:hellingerS}
\hellingerS{p, q} = 1- \sum_{j}\sqrt{p_j\cdot q_j}.
\end{align}

It follows from \eqref{eq:churn-random-collision} that
\begin{align}
\churnR{w_1, w_2} &= 1 - \mathbb{E}_{\X}\big[\sum_{j \in \mathscr{Y}} f(\X; w_1) f(\X; w_2)\big] \nonumber \\
& \geq 1 - \mathbb{E}_{\X}\big[\sum_{j \in \mathscr{Y}} \sqrt{f(\X; w_1) f(\X; w_2)}\big] \nonumber \\
& = \mathbb{E}_{\X}\big[\hellingerS{f(\X; w_1), f(\X; w_2)}\big].
\end{align}
Now, using the relationship between the Hellinger distance and the total variation distance $\TV(p,q) = \frac{1}{2}\cdot\sum_j|p_j - q_j|$, i.e., 
$$
\hellingerS{p, q} \leq \TV(p, q) \leq \sqrt{2}\hellinger{p, q},
$$
we obtain that 
\begin{align}
\churnR{w_1, w_2} \geq \frac{1}{2}\cdot \mathbb{E}_{\X}\big[\TV^2(f(\X; w_1), f(\X; w_2))\big].
\end{align}
%\end{remark}

%
%\begin{remark}
A trivial upper bound is
$$ \churnR{w_1, w_2} \leq 1 - \mathbb{E}_{\X}\big[ f(\X;w_1)^{\mathrm{T}} f(\X;w_1) \big]  + \mathbb{E}_{\X}\big[ D_{\mathrm{TV}}( f(\X;w_1) \| f(\X;w_2) ) \big]. $$
Observe that this bound is tight when $w_1 = w_2$, since here the churn is just the collision probability, 
i.e.,
$1 - \mathbb{E}_{\X}\big[ f(\X;w_1)^{\mathrm{T}} f(\X;w_1) \big]$.
In other words, the total variation distance between $f(\X;w_1)$ and $f(\X;w_2)$ bounds the \emph{churn regret}.

To see why this is true, observe that for any probability vectors $a, b$,
\begin{align}
    - a^{\mathrm{T}} b &= a^{\mathrm{T}} (-b) \nonumber \\
    &= a^{\mathrm{T}} (a-b-a) \nonumber \\
    &= - a^{\mathrm{T}} a  + a^{\mathrm{T}} (a-b) \nonumber \\
    &\leq - a^{\mathrm{T}} a  + \| a \|_{\infty} \cdot \| a-b \|_1 \nonumber \text{ by H\"{o}lder's inequality } \\
    &\leq - a^{\mathrm{T}} a  + \| a - b \|_1 \text{ since } a \text{ is a distribution } \nonumber \\
    &= - a^{\mathrm{T}} a  + D_{\mathrm{TV}}( a \| b ).
\end{align}
%\end{remark}
\end{proof}
